# Supplementary material for: Control Synthesis for Stability and Safety by Differential Complementarity Problem
Source: arXiv:2210.01978 source file (2022-12-09)
Supplement: Supplementary file 2 [file Old_appendix.tex]

%%%%%%%%%%%%%%%%%%%%%%%%%%%%%%%%%%%%%%%%%%%%%%%%%%%%%%%%%%%%%%%%%%%%
	\section{APPENDIX}
	\label{sec: appendix}
	
	\subsection{Generalized DCP Formulation}
	Let's consider a more general system dynamics:
	%
	\begin{equation}
	\label{dynamics: general}
		\dot{\bfx} = \bfF(\bfx) + \bfg(\bfx)\bfu,
	\end{equation}
	%
	where $\bfF(\bfx)$ is a stabilizing system and $\bfx \in \bbR^n, \bfg(\bfx) \in \bbR^{n \times m}, \bfu \in \bbR^m$.
	However, it will fail if we attempt to employ safety by directly reformulate the system above into a DCP, so we make the following modifications:
	%
	\begin{equation}
	\label{baru}
		\bfu = \bfW\bar{u},
	\end{equation}
	%
	where $\bfW \in \bbR^m, \bar{u} \in \bbR$.
	Thus, we have the following DCP:
	\begin{equation}
	\label{DCP: generalized}
	\begin{aligned}
		&\dot{\bfx} = \bfF(\bfx) + \bfg(\bfx)\bfW\bar{u}, \\
		\mathrm{s.t.} \, \, & 0 \leq \bar{u} \perp \mathcal{L}_{\bfF}h_0 + \mathcal{L}_{\bfg}h_0 \cdot \bfW\bar{u} + \alpha(h_0)  \geq 0.
	\end{aligned}
	\end{equation}
	%
	with its solution given by:
	%
	\begin{equation}
	\label{DCP: sol}
	\begin{aligned}
		&\bar{u} = \left\{
		\begin{aligned}
			&0, \ &\text{if} \ \mathcal{L}_{\bfF}h_0 + \alpha(h_0) \geq 0, \\
			&f_{\bar{u}}(\bfx), \ &\text{if} \ \mathcal{L}_{\bfF}h_0 + \alpha(h_0) < 0,
		\end{aligned} \right.
	\end{aligned}
	\end{equation}
	%
	where $f_{\bar{u}}(\bfx)$ is given by:
	%
	\begin{align}\label{DCP: sol_f}
		f_{\bar{u}}(\bfx) = -(\mathcal{L}_{\bfg}h_0 \cdot \bfW)^{-1}(\mathcal{L}_{\bfF}h_0 + \alpha(h_0)).
	\end{align}
	%
	In order to satisfy the condition $\bar{u} \geq 0$, we want to make sure that $\mathcal{L}_{\bfg}h_0 \cdot \bfW > 0$. Thus, a naive choice of $\bfW$ would be: $\bfW = (\mathcal{L}_{\bfg}h_0)^T$.
	\subsection{Combining CLF and CBF as a DCP:} This part shows how I combine CLF ($V$) and CBF ($h_0$) as a DCP and justify my observation that this approach will not introduce any local equilibrium other than the origin.
	We consider the following control affine nonlinear dynamic system:
	%
	\begin{equation}
	\label{dynamics: ctrl_aff}
	\dot{\bfx} = \bff(\bfx) + \bfg(\bfx)\bfu,
	\end{equation}
	%
	Just like what we did in previous section, the control input $\bfu$ has the following structure:
	%
	\begin{equation}
	\label{struc: bfu}
		\bfu = \bfW_l\bar{u}_l + \bfW_h\bar{u}_h,
	\end{equation}
	%
	where $\bfW_l, \bfW_h \in \bbR^m, \bar{u}_l, \bar{u}_h \in \bbR$.
	We have the following DCP:
	%
	\begin{equation}
	\label{DCP: combined}
	\begin{aligned}
		&\dot{\bfx} = \bff(\bfx) + \bfg(\bfx)[\bfW_l\bar{u}_l + \bfW_h\bar{u}_h], \\
		\mathrm{s.t.} \, \, & 0 \leq \bar{u}_l \perp -\mathcal{L}_{\bff}V - \mathcal{L}_{\bfg}V \cdot \bfW_l\bar{u}_l - \alpha(V)  \geq 0, \\
		& 0 \leq \bar{u}_h \perp \mathcal{L}_{\bff}h_0 + \mathcal{L}_{\bfg}h_0 \cdot [\bfW_l\bar{u}_l + \bfW_h\bar{u}_h] + \alpha(h_0)  \geq 0.
	\end{aligned}
	\end{equation}
	%
	If we have:
	%
	\begin{equation}
	\label{equi: local}
		\mathbf{0} = \bff(\bfx) + \bfg(\bfx)[\bfW_l\bar{u}_l + \bfW_h\bar{u}_h], \quad \forall \bfx \neq \mathbf{0}, 
	\end{equation}
	%
	then a local equilibrium has been introduced.
	Now consider our DCP formulation \eqref{DCP: combined}, which has four possible combinations of solutions. 
	\begin{itemize}
		\item[*] $\bar{u}_l = 0, \bar{u}_h = 0$ Under this condition, if we have $\bff(\bfx) = \mathbf{0}$, then a local equilibrium has been introduced. However, the CLF constraint: $-\mathcal{L}_{\bff}V - \alpha(V)  \geq 0$ requires $\bff(\bfx)$ to be nonzero otherwise it is violated.
		\item[*] $\bar{u}_l = 0, \bar{u}_h \neq 0$ Under this condition, if we have $\mathbf{0} = \bff(\bfx) + \bfg(\bfx)\bfW_h\bar{u}_h$, then a local equilibrium has been introduced. However, $\bar{u}_h \neq 0$ requires the CBF constraint: $\mathcal{L}_{\bff}h_0 + \mathcal{L}_{\bfg}h_0 \cdot \bfW_h\bar{u}_h + \alpha(h_0) = 0$ requires $\bff(\bfx) + \bfg(\bfx)\bfW_h\bar{u}_h$ to be nonzero otherwise it is violated, except $\alpha(h_0) = 0$.
		\item[*] $\bar{u}_l \neq 0, \bar{u}_h = 0$ Under this condition, if we have $\mathbf{0} = \bff(\bfx) + \bfg(\bfx)\bfW_l\bar{u}_l$, then a local equilibrium has been introduced. Apparently this could not happen otherwise we will have the CLF constraint becomes: $- \alpha(V)  \geq 0$, which could not hold unless $V = 0$.
		\item[*] $\bar{u}_l \neq 0, \bar{u}_h \neq 0$ Under this condition, if we have $\mathbf{0} = \bff(\bfx) + \bfg(\bfx)[\bfW_l\bar{u}_l + \bfW_h\bar{u}_h]$, then a local equilibrium has been introduced. However, $\bar{u}_h \neq 0$ requires the CBF constraint: $\mathcal{L}_{\bff}h_0 + \mathcal{L}_{\bfg}h_0 \cdot [\bfW_l\bar{u}_l + \bfW_h\bar{u}_h] + \alpha(h_0) = 0$ requires $\bff(\bfx) + \bfg(\bfx)[\bfW_l\bar{u}_l + \bfW_h\bar{u}_h]$ to be nonzero otherwise it is violated, except $\alpha(h_0) = 0$.
	\end{itemize}
	However, local equilibrium still exists if we have: $\alpha(h_0) = 0, \bfx \neq \mathbf{0}$, here I present a sketch on how to deal this problem.
	Define $\bff(\bfx) + \bfg(\bfx)[\bfW_l\bar{u}_l + \bfW_h\bar{u}_h] = \bfe(\bfx)$ and we have the following DCP:
	%
	\begin{equation}
	\label{DCP: final}
	\begin{aligned}
		&\dot{\bfx} = \bff(\bfx) + \bfg(\bfx)[\bfW_l\bar{u}_l + \bfW_h\bar{u}_h + \bfx^T\bfx \bfW_{h_{null}}\bar{\bfu}_{h_{null}}], \\
		\mathrm{s.t.} \, \, & 0 \leq \bar{u}_l \perp -\mathcal{L}_{\bff}V - \mathcal{L}_{\bfg}V \cdot \bfW_l\bar{u}_l - \alpha(V)  \geq 0, \\
		& 0 \leq \bar{u}_h \perp \mathcal{L}_{\bff}h_0 + \mathcal{L}_{\bfg}h_0 \cdot [\bfW_l\bar{u}_l + \bfW_h\bar{u}_h] + \alpha(h_0)  \geq 0, \\
		& \mathbf{0} \leq \bar{\bfu}_{h_{null}} \perp \bfI_{n-1} \otimes (\bfe(\bfx)^T\bfe(\bfx) - \epsilon) + \bar{\bfu}_{h_{null}} \geq \mathbf{0}.
	\end{aligned}
	\end{equation}
	%
	where $\bfW_{h_{null}} = null(\mathcal{L}_{\bfg}h_0) \Rightarrow \mathcal{L}_{\bfg}h_0 \cdot \bfW_{h_{null}} = \mathbf{0}^T_{n-1}$ and $\epsilon$ arbitrarily small.
	The motivation is to formulate another DCP constraint in addition to what we have in equation \eqref{DCP: combined} dedicated to the scenario where our robot is operating on the boundary (virtual boundary if we have $h_0 = h_{true} + \tau$) of the obstacle.
	\begin{figure}[ht]
		\centering
		\includegraphics[width=7cm]{cortes_example.eps}
		\caption{Example from Cortes} \label{Local Equilibrium}
	\end{figure}
	\textcolor{red}{Some extra assumptions should be put on $g(\bfx)$ otherwise there have no means to address this issue.}

 %%%%%%%%%%%%%%%%%%%%%%%%%%%%%%%%%%%%%%%%%%%%%%%%%%%%%%%%%%%%%%%
 \subsection{Some Definitions and Propositions}
\begin{definition}[Incompatible Points]
	We consider points on the boundary of our obstacle where CBF constraints are inactive and vector field generated by the unforced system \eqref{dynamics: Sys_unforced}  is in the opposite direction of our extra forcing term. We denote the collection of such points as $\bar{\calU}$ defined as follows:
	\begin{equation}
	\label{criteria: inco_points}
		\bar{\calU} \coloneqq \{ \bfx \in \partial \calC: \dot{\bar{\bfx}}^{\top} \cdot 	\bfG(\bfx)\bfw_p < 0, \bar{u}_h(\bfx) = 0 \}
	\end{equation}
\end{definition}
%
\begin{proposition} The modified CLF-CBF-QP proposed in \cite{tan2021undesired} is equivalent to the following weighted CLF-CBF-QP:
	%
	\begin{equation}\label{controller: M-CLF-CBF-QP}
		\begin{aligned}
			\bfu(\bfx) = & \argmin_{(\bfu, \delta) \in \bbR^{m+1}} \frac{1}{2} || \bfu - \bfr(\bfx) ||_2^2 + \frac{1}{2} p \delta^2 \\
			\mathrm{s.t.} \, \, &\calL_{\bff} V(\bfx) + \calL_{\bfG} V(\bfx) \bfu + \alpha_l(V) \leq \delta \\
			&\calL_{\bff} h(\bfx) + \calL_{\bfG} h(\bfx) \bfu \geq -\alpha_h(h) 
		\end{aligned}
	\end{equation}
	%
	where $\bfr(\bfx) \in K_{clf}$ and locally Lipschitz.
	\begin{proof}
		Substitute $\bfu = \bfu' + \bfr(\bfx)$ and the result follows. By doing so, the following scenario has been eliminated: CLF constraint is active while CBF constraint is inactive. Since $\bfr$ is already a stabilizing controller satisfying CLF constraint, inactive CBF constraint means that there is no impact on the resulted controller generated by \eqref{controller: M-CLF-CBF-QP} and we have $\bfu = \bfr$, which means that CLF constraints should be inactive. Thus, local equilibria in $\textrm{Int}(\calC) \partial \calC$ has been eliminated.
	\end{proof}
\end{proposition}

Another method is to take $k$ as a function of $\bar{u}_h$ and we will have the following structure: $k = \frac{k'}{\bar{u}_h}$, then $\bar{u}_h k \bfG(\bfx) \bfw_p = k'\bfG(\bfx) \bfw_p$ which is independent of $\bar{u}_h$. 

%%%%%%%%%%%%%%%%%%%%%%%%%%%%%%%%13/09/2022%%%%%%%%%%%%%%%%%%%%%%%%%%%%%%%
\section{Appendix}
This method is to make $k$ a function of $\bar{u}_h$ and takes the following structure: $k = \frac{k'}{\bar{u}_h}$, then we have the $\bar{u}_h k \bfG(\bfx) \bfw_p$ term equals to $k'\bfG(\bfx) \bfw_p$ and independent of $\bar{u}_h$. As a result, by using this method, the system dynamics has been changed and we should consider the following system:
%
\begin{equation}
	\label{dynamics: Forced_sys}
	\dot{\bfx} = \bff'(\bfx) + \bfG(\bfx)\bfu
\end{equation}
%
with $\bff'(\bfx) = \bff(\bfx) + k'\bfG(\bfx) \bfw_p$. 
And we modify the original DCP formulation accordingly to reflect the changes:
%
\begin{subequations}
	\label{DCP: forced-form}
	\begin{align}
		&\dot{\bfx} = \bff'(\bfx) + \bfG(\bfx)[\bfw_l\bar{u}'_l + \bfw_h\bar{u}'_h], \ \forall \bfx \in \bbR^n \nonumber \\
		\mathrm{s.t.} \, \, & 0 \leq \bar{u}'_l \perp -\bfF'_V(\bfx) - \mathcal{L}_{\bfG}V \cdot \bfw_l\bar{u}'_l \geq 0, \label{DCP_forced: CLC} \\
		& 0 \leq \bar{u}'_h \perp \bfF_h(\bfx) + \mathcal{L}_{\bfG}h \cdot [\bfw_l\bar{u}'_l + \bfw_h\bar{u}'_h] \geq 0 \label{DCP_forced: CBC}
	\end{align}
\end{subequations}
%
where $\bfw_l = -\mathcal{L}_{\bfG}V^{\top}, \bfw_h = \mathcal{L}_{\bfG}h^{\top}$ and $\bfF'_V(\bfx) = \mathcal{L}_{\bff'}V + \alpha_l(V)$. Notice that we have $\mathcal{L}_{\bff'}h = \nabla h \cdot [\bff(\bfx) + k'\bfG(\bfx) \bfw_p] = \nabla h \cdot \bff(\bfx) = \mathcal{L}_{\bff}h$ due to the fact that $\mathcal{L}_{\bfG}h \cdot \bfw_p = 0$, as a result we have $\bfF_h(\bfx)$ unchanged comparing to \eqref{DCP: BQ-form}.
According to Proposition~\ref{prop: local_equi}, our DCP system \eqref{DCP: forced-form} only admits local equilibria on the boundary of the obstacle with CBC constraint \eqref{DCP_forced: CBC} active. Hence we consider the following two cases:

\textbf{Case 1.} CLC constraint \eqref{DCP_forced: CLC} inactive: In this case, if we have:
%
\begin{equation}
	\label{le_forced_sys: clc_i}
	\mathbf{0} = \bff'(\bfx) + \bfG(\bfx)\bfw_h\bar{u}'_h
\end{equation}
%
where $\bar{u}'_h$ is given by solving \eqref{DCP_forced: CBC}: $\bar{u}'_h = -\frac{\mathcal{L}_{\bff}h}{\| \mathcal{L}_{\bfG}h \|^2_2}$, then local equilibria exists. Substituting $\bff'(\bfx)$ and $\bar{u}'_h$ into equation above and we have:
%
\begin{equation}
	\label{le_forced_sol: clc_i}
	k'\bfG(\bfx) \bfw_p = \frac{\mathcal{L}_{\bff}h}{\| \mathcal{L}_{\bfG}h \|^2_2} \bfG(\bfx)\mathcal{L}_{\bfG}h^{\top} - \bff(\bfx).
\end{equation}
%
Define:
%
\begin{equation}
	N_1 \coloneqq \sup_{\bfx \in \calU^i_{\calC}} \| \bfg_i(\bfx) \|, \ N_2 \coloneqq \inf_{\bfx \in \calU^i_{\calC}} \| \bfG(\bfx) \bfw_p \| \notag
\end{equation}
%
with $\calU^i_{\calC} \coloneqq \{ \bfx \in \partial \calC: \bar{u}'_h > 0, \bar{u}'_l = 0, \bfg_i(\bfx) \neq \mathbf{0}, \| \bfg_i(\bfx) \|_2 \| \bfG(\bfx) \bfw_p \|_2 + \bfg_i(\bfx)^{\top} \bfG(\bfx) \bfw_p = 0 \}$ and $\bfg_i(\bfx) = \bff(\bfx) + \bar{u}'_h \bfG(\bfx) \mathcal{L}_{\bfG}h^{\top}$.

\textbf{Case 2.} CLC constraint \eqref{DCP_forced: CLC} active: In this case, if we have:
%
\begin{equation}
	\label{le_forced_sys: clc_a}
	\mathbf{0} = \bff'(\bfx) + \bfG(\bfx)[\bfw_l\bar{u}'_l + \bfw_h\bar{u}'_h],
\end{equation}
%
where $\bar{u}'_l$ is given by solving \eqref{DCP_forced: CLC}: $\bar{u}'_l = \frac{\mathcal{L}_{\bff'}V + \alpha_l(V)}{\| \mathcal{L}_{\bfG}V \|_2^2} = f_l(\bfx) + k'\frac{\calL_{\bfG}V\bfw_p}{\| \mathcal{L}_{\bfG}V \|_2^2}$ and $\bar{u}'_h$ is given by solving \eqref{DCP_forced: CBC}: $\bar{u}'_h = -\frac{\mathcal{L}_{\bff}h - \mathcal{L}_{\bfG}h \mathcal{L}_{\bfG}V^{\top} \bar{u}'_l }{ \| \mathcal{L}_{\bfG}h \|_2^2 } = f'_h(\bfx) + k'\frac{\mathcal{L}_{\bfG}h \mathcal{L}_{\bfG}V^{\top} \mathcal{L}_{\bfG}V}{\| \mathcal{L}_{\bfG}h \|^2_2 \| \mathcal{L}_{\bfG}V \|_2^2}\bfw_p$, then local equilibria exists.
Substituting $\bff'(\bfx)$ and $\bar{u}'_l, \bar{u}'_h$ into equation above and we have:
%
%\begin{equation}
%\label{le_forced_sol: clc_a}
%\begin{aligned}
%&\bff(\bfx) + k'\bfG(\bfx) \bfw_p - \frac{\mathcal{L}_{\bff}h}{\| \mathcal{L}_{\bfG}h 	%\|_2^2}\bfG(\bfx)\mathcal{L}_{\bfG}h^{\top} = \\
%&\bar{u}'_l \bfG(\bfx) [\mathcal{L}_{\bfG}V^{\top} - \frac{\mathcal{L}_{\bfG}h \mathcal{L}_{\bfG}V^{\top}}{\| %\mathcal{L}_{\bfG}h \|^2_2}\mathcal{L}_{\bfG}h^{\top}].
%\end{aligned}
%\end{equation}
%
%In order to separate $k'$, we rewrite equation above as:
%
\small
\begin{equation}
	\label{le_forced_sol: k'}
	\begin{aligned}
		&k'\bfG(\bfx) \bfw_p -  k'\frac{\calL_{\bfG}V\bfw_p}{\| \mathcal{L}_{\bfG}V \|_2^2} \bfG(\bfx) [\mathcal{L}_{\bfG}V^{\top} - \frac{\mathcal{L}_{\bfG}h \mathcal{L}_{\bfG}V^{\top}}{\| \mathcal{L}_{\bfG}h \|^2_2}\mathcal{L}_{\bfG}h^{\top}] = \\
		&k'\bfG(\bfx)[ \bfI_{m \times m} - \frac{\calL_{\bfG}V^{\top} \mathcal{L}_{\bfG}V}{\| \mathcal{L}_{\bfG}V \|_2^2} + \frac{\mathcal{L}_{\bfG}h^{\top} \mathcal{L}_{\bfG}h \mathcal{L}_{\bfG}V^{\top} \mathcal{L}_{\bfG}V}{\| \mathcal{L}_{\bfG}h \|^2_2 \| \mathcal{L}_{\bfG}V \|_2^2} ]\bfw_p = \\
		&k'\bfG(\bfx)\bfK(\bfx)\bfw_p = -\bff(\bfx) + \bfG(\bfx) [f_l(\bfx) \mathcal{L}_{\bfG}V^{\top} - f'_h(\bfx) \mathcal{L}_{\bfG}h^{\top}]
	\end{aligned}
\end{equation}
\normalsize
%
Define:
%
\begin{equation}
	N_3 \coloneqq \sup_{\bfx \in \calU^a_{\calC}} \| \bfg_a(\bfx) \|, \ N_4 \coloneqq \inf_{\bfx \in \calU^a_{\calC}} \| \bfG(\bfx) \bfK(\bfx) \bfw_p \| \notag,
\end{equation}
%
with $\calU^a_{\calC} \coloneqq \{ \bfx \in \partial \calC: \bar{u}'_h > 0, \bar{u}'_l > 0, \bfg_a(\bfx) \neq \mathbf{0}, \| \bfg_a(\bfx) \|_2 \| \bfG(\bfx) \bfK(\bfx) \bfw_p \|_2 + \bfg_a(\bfx)^{\top} \bfG(\bfx) \bfK(\bfx) \bfw_p = 0 \}$ and $\bfg_a(\bfx) = \bff(\bfx) + \bfG(\bfx) [-f_l(\bfx) \mathcal{L}_{\bfG}V^{\top} + f'_h(\bfx) \mathcal{L}_{\bfG}h^{\top}]$. 

If we could find a finite constant $k' > \max(\frac{N_1}{N_2}, \frac{N_3}{N_4})$ then we will have every local equilibria removed. However, such $k'$ is not always available since $N_4$ could be zero. Due to the assumption that $\bfG(\bfx)$ has full column rank, $N_4 = 0 \iff \bfK(\bfx) \bfw_p = \mathbf{0}, \bfx \in \calU^a_{\calC}$. We consult the following proposition to determine the conditions under which $\bfK(\bfx) \bfw_p$ would be zero.
\begin{proposition}
	Consider non-zero vectors $\bfa, \bfb \in \bbR^{m \times 1}$ with $m \geq 2$ and $\bfc \in \textrm{null}(\bfb)$. The following equation holds 
	\begin{equation}
		[\bfI_{m \times m} - \frac{\bfa\bfa^{\top}}{\bfa^{\top}\bfa} + \frac{\bfb\bfb^{\top}\bfa\bfa^{\top}}{\bfb^{\top}\bfb\bfa^{\top}\bfa}]\bfc = \mathbf{0}
	\end{equation}
	if and only if we have $\bfa$ and $\bfc$ linearly dependent. 
	\begin{proof}
		We could write $\bfa$ in the following form: $\bfa = a\bfb + \sum_{i = 1}^{m-1}b_i\bfb_i^{\perp}$ where $\bfb_i^{\perp}$ forms an orthonormal basis of the null space of $\bfb$ and with out loss of generality, we assume $\bfc = \bfb_k^{\perp}$. Now we have: $\frac{\bfb\bfb^{\top}\bfa\bfa^{\top}}{\bfb^{\top}\bfb\bfa^{\top}\bfa} = a \frac{\bfb\bfa^{\top}}{\bfa^{\top}\bfa}$ and $\bfa^{\top}\bfc = b_k$. As a result we have the following equation:
		$(a^2 \| \bfb \|_2^2 + \sum_{i = 1}^{m-1}b_i^2) \bfb_k^{\perp} - b_k\bfa + ab_k\bfb = (a^2 \| \bfb \|_2^2 + \sum_{i = 1}^{k-1}b_i^2 + \sum_{j = k + 1}^{m-1}b_j^2) \bfb_k^{\perp} - b_k(\sum_{i = 1}^{k-1}b_i\bfb_i^{\perp} + \sum_{j = k + 1}^{m-1}b_j\bfb_j^{\perp}) = \mathbf{0}$. Since we need to have at least one $a, b_i \neq 0$, the only solution to the equation above is $a = 0$ and $b_i = 0, \ \forall i \neq k$. Thus the result follows.
	\end{proof}
\end{proposition}
Also, we should notice that $\bfg_a(\bfx) \neq \mathbf{0}$ in this case at all points where we have $\mathcal{L}_{\bfG}V^{\top}$ and $\bfw_p$ linearly dependent. Since we have: $\nabla V \cdot \bfg_a(\bfx) = \mathcal{L}_{\bff}V + f'_h(\bfx) \mathcal{L}_{\bfG}V \mathcal{L}_{\bfG}h^{\top} - f_l(\bfx) \| \mathcal{L}_{\bfG}V \|_2^2$ and due to the fact that $\mathcal{L}_{\bfG}V^{\top}$ and $\bfw_p$ linearly dependent implies $\mathcal{L}_{\bfG}V^{\top} \in \textrm{null}(\mathcal{L}_{\bfG}h)$, equation above becomes $\nabla V \cdot \bfg_a(\bfx) = \mathcal{L}_{\bff}V - f_l(\bfx) \| \mathcal{L}_{\bfG}V \|_2^2$ and if we substitute $f_l(\bfx)$ we will have: $\nabla V \cdot \bfg_a(\bfx) = -\alpha_l(V)$, indicating that $\bfg_a(\bfx) \neq \mathbf{0}$.

So, if we could find a locally Lipschitz $\bfw_p$ such that $\mathcal{L}_{\bfG}V^{\top}$ and $\bfw_p$ are linearly independent for all $\bfx \in \calU^a_{\calC}$, then we could find a finite constant $k'$ such that $k' > \max(\frac{N_1}{N_2}, \frac{N_3}{N_4})$. And as a result, our DCP system \eqref{DCP: forced-form} admits no local equilibria with such $k'$. 

However, if we have $N_4 = 0$, then a finite constant $k'$ will not be available, in that case, instead of using $k' > \max(\frac{N_1}{N_2}, \frac{N_3}{N_4})$, we use $k' > \frac{N_3}{\nu'} \geq \frac{N_1}{N_2}$ where $\nu'$ is a user specified constant. Using such a $k'$, local equilibria on $\partial \calC$ will be confined to the follow set:  $\calQ' \coloneqq \{ \bfx \in \partial \calC: \bar{u}'_h > 0, \| \bfg_a(\bfx) \|_2 \| \bfG(\bfx) \bfK(\bfx) \bfw_p \|_2 + \bfg_a(\bfx)^{\top} \bfG(\bfx) \bfK(\bfx) \bfw_p = 0, \bfg_a(\bfx) \neq \mathbf{0}, 0< \| \bfG(\bfx) \bfK(\bfx) \bfw_p \|_2 \leq \nu' \}$. And we could make $\calQ'$ shrink to the following set: $\calS'_i \coloneqq \{  \bfx \in \partial \calC: \bar{u}'_h > 0, \| \mathcal{L}_{\bfG}V \|_2 \| \bfw_p \|_2 - | \mathcal{L}_{\bfG}V \cdot \bfw_p | = 0,  \| \bfg_a(\bfx) \|_2 \| \bfG(\bfx) \bfK(\bfx) \bfw_p \|_2 + \bfg_a(\bfx)^{\top} \bfG(\bfx) \bfK(\bfx) \bfw_p = 0, \bfg_a(\bfx) \neq \mathbf{0} \}$ by increasing $k'$ (decreasing $\nu'$). As a result, we only need to make sure $\calS'_i$ will not intersect with our desired trajectory on $\partial \calC$, otherwise, we could do nothing to avoid being stuck at a local equilibrium.
%
\begin{figure}[t]
	\centering
	\includegraphics[width=\linewidth]{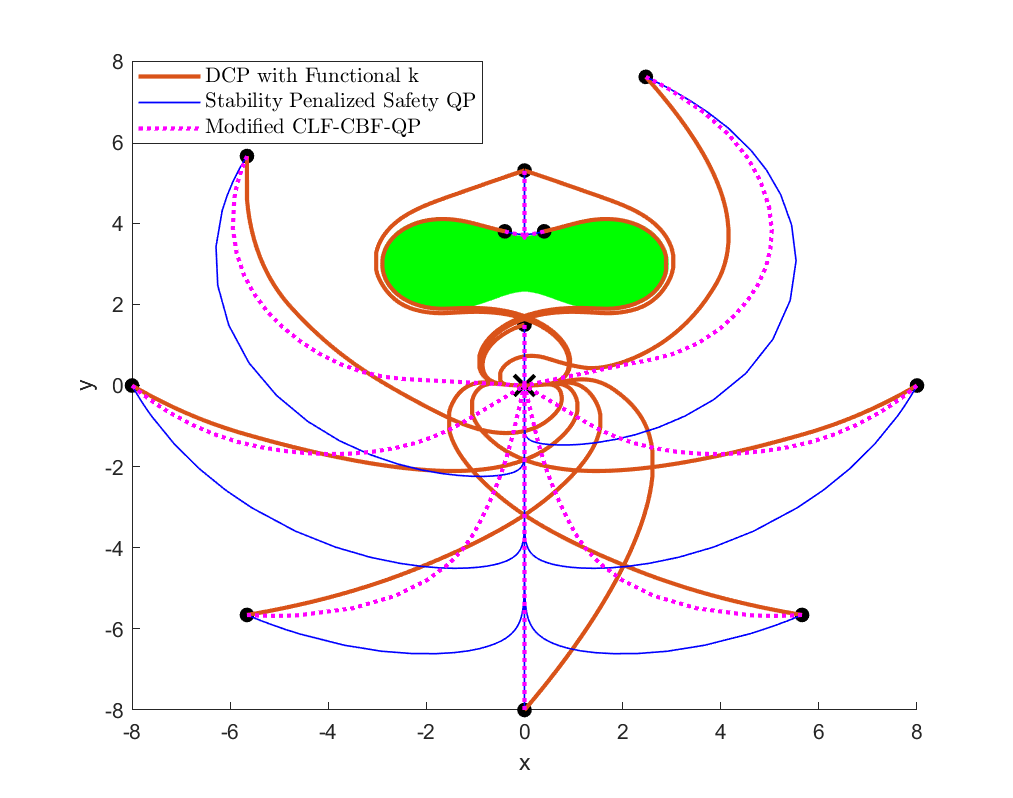}
	\caption{CLF-CBF-DCP with a functional $k=\frac{2}{\bar{u}_h}$ used to avoid concave obstacle (green) starting from different initial conditions. We notice that both modified CLF-CBF-QP and stability penalized safety QP gets stuck at a boundary local equilibrium ($0,3.65$) starting at ($\pm0.5, 4$) and ($0,5.3$) due to the concaveness of the obstacle. Although in this case we always have $N_4 = 0$, our CLF-CBF-DCP with a functional $k$ still ensures both safety and stabilized to the origin, which is due to the fact that $\calS'_i$ is not intersecting with our trajectory. We should also note that the our CLF-CBF-DCP with a functional $k$ generates distinct trajectories comparing to a constant $k$. }
	\label{fig: con_fk}
\end{figure}
%
\begin{remark}
	One should notice that in \eqref{DCP: forced-form} the extra forcing term $\bfG(\bfx)\bfw_p$ appears in our system dynamics as a permanent control input and as a result, the original drift term $\bff(\bfx)$ has been changed to $\bff'(\bfx)$. So, one should not use this method if the original drift term is of particular interest.
\end{remark}

\subsection{Connecting DCP and QP Based Methods}
%\TODO{In this section, we abuse the use of terminology equivalent. In our paper, when we say that the two systems are equivalent or attain equivalency, we mean that they receive the same control input at the same state.}
We first notice that the solution of control $\bfu$ by our CLF-CBF-DCP is equivalent to the one by CBF-QP if we take the \textit{naive choice} of $\bfw_l, \bfw_h$ and set $\bfr(\bfx) = -( \frac{F_V(\bfx)}{\| \mathcal{L}_{\bfG}V(\bfx) \|_2^2} )_+ \mathcal{L}_{\bfG}V(\bfx)^{\top}$ in \eqref{controller: CBF-QP}, which is the pointwise minimum-norm controller in \cite{pol2022roa}. However, if one wants to use a given reference stabilizing control input $\bfr(\bfx)$ in CBF-QP other than the solution of \eqref{DCP: CLC}, a different DCP must be formulated to attain equivalency as shown in the following proposition.
\begin{proposition}\label{DCP: BQ-Equi} 
Consider the following DCP system:
	%
	\begin{subequations}
		\label{DCP: CBF-QP_equi}
		\begin{align}
			&\dot{\bfx} = \bff(\bfx) + \bfG(\bfx)[\bfr(\bfx) + \bfw_h\bar{u}_h], \nonumber \\
			\mathrm{s.t.} \, \, 
			& 0 \leq \bar{u}_h \perp F_h(\bfx) + \mathcal{L}_{\bfG}h(\bfx) \cdot [\bfr(\bfx) + \bfw_h\bar{u}_h] \geq 0 \label{CBC: DBQ}
		\end{align}
	\end{subequations}
	%
	where $\bfw_h = \mathcal{L}_{\bfG}h(\bfx)^{\top}$. The resulting feedback controller $\bfu = \bfr(\bfx) + \bfw_h \bar u_h$ using the solution to \eqref{CBC: DBQ} is equivalent to the controller obtained by CBF-QP in Proposition \ref{sol: QP} for arbitrary $\bfr(\bfx)$.  
	\begin{proof}
		The solution to \eqref{CBC: DBQ} is easily obtained as follows:
		\begin{equation}
			\label{sol: bu_h_DBQ}
			\bar{u}_h = \left(-\frac{\calL_{\bff} h(\bfx) + \calL_{\bfG} h(\bfx)\bfr(\bfx) + \alpha_h(h)}{\| \calL_{\bfG} h(\bfx) \|_2^2} \right)_+
		\end{equation}
		Thus, we have $\bfu = \bfr(\bfx) + \bfw_h\bar{u}_h = \bfr(\bfx) + \bar{u}_h \calL_{\bfG} h(\bfx)^{\top}$, which is identical to the solution for CBF-QP formulation in Proposition \ref{sol: QP}.
	\end{proof}
\end{proposition}
Furthermore, we consider the following CLF-CBF-QP:
%
\begin{equation}\label{controller: CLF-CBF-QP}
	\begin{aligned}
		\bfu(\bfx) = & \argmin_{(\bfu, \delta) \in \bbR^{m+1}} \frac{1}{2} || \bfu ||_2^2 + \frac{1}{2} p \delta^2 \\
		\mathrm{s.t.} \, \, &\calL_{\bff} V(\bfx) + \calL_{\bfG} V(\bfx) \bfu + \alpha_l(V) \leq \delta \\
		&\calL_{\bff} h(\bfx) + \calL_{\bfG} h(\bfx) \bfu \geq -\alpha_h(h) 
	\end{aligned}
\end{equation}
%
An equivalent solution with \eqref{controller: CLF-CBF-QP} can also be formulated as a DCP shown below:
\begin{proposition}\label{DCP: LBQ-Equi} 
	%
	Consider the following DCP: 
	\begin{subequations}
		\label{DCP: LBQ-form}
		\begin{align}
			\dot{\bfx} = \bff(\bfx) + &\bfG(\bfx)[- \mathcal{L}_{\bfG}V(\bfx)^{\top}\bar{u}_l + \mathcal{L}_{\bfG}h(\bfx)^{\top}\bar{u}_h] \nonumber \\
			\mathrm{s.t.} \, \,  0 \leq \bar{u}_l &\perp -\calL_{\bff} V(\bfx) - \alpha_l(V) - \mathcal{L}_{\bfG}V(\bfx) \mathcal{L}_{\bfG}h(\bfx)^{\top}\bar{u}_h  \nonumber \\
			&+ \left[\mathcal{L}_{\bfG}V(\bfx) \mathcal{L}_{\bfG}V(\bfx)^{\top} + \frac{1}{p} \right]\bar{u}_l  \geq 0, \label{DCP_LBQ: CLC} \\
			0 \leq \bar{u}_h &\perp \calL_{\bff} h(\bfx) + \alpha_h(h) - \mathcal{L}_{\bfG}h(\bfx) \mathcal{L}_{\bfG}V(\bfx)^{\top}\bar{u}_l \nonumber \\
			&+ \mathcal{L}_{\bfG}h(\bfx) \mathcal{L}_{\bfG}h(\bfx)^{\top}\bar{u}_h \geq 0 \label{DCP_LBQ: CBC}
		\end{align}
	\end{subequations}
	The resulting feedback controller $\bfu = - \mathcal{L}_{\bfG}V(\bfx)^{\top}\bar{u}_l + \mathcal{L}_{\bfG}h(\bfx)^{\top}\bar{u}_h$ is equivalent to the solution to CLF-CBF-QP in \eqref{controller: CLF-CBF-QP}. 
	%
	\begin{proof}
		The proof follows by evaluating the KKT conditions of CLF-CBF-QP \eqref{controller: CLF-CBF-QP}. First we obtain the closed-form expression of $\bfu$ w.r.t. Lagrange multipliers $\lambda_1, \lambda_2$ by solving $\frac{\partial \calL}{\partial \bfu} = 0$, then we obtain the close form expression of $\delta$ w.r.t. Lagrangian multiplier $\lambda_1$ by solving $\frac{\partial \calL}{\partial \delta} = 0$. Substituting them into complementary constraints leads to the closed-form solution of $\bfu$ by CLF=CBF-QP, which is equivalent to the resulting feedback controller given in the proposition. Note that in \eqref{DCP: LBQ-form} the variables $\bar{u}_l$ and $\bar{u}_h$ actually serve as Lagrangian multipliers $\lambda_1$ and $\lambda_2$ in CLF-CBF-QP respectively.
	\end{proof}
\end{proposition}
In this section we have verified that QP-based methods through Propositions~\ref{DCP: BQ-Equi}, \ref{DCP: LBQ-Equi} can be also formulated as DCP with equivalent solution. In the following section, we focus on the CLF-CBF-DCP formulation and demonstrate that how to choose $\bfw_h$ other than the \textit{naive choice} to fully exploit the advantage of our formulation.

Since we can make $\calQ$ shrinking to $\calS_i$, there might be an issue only if we wish to drive the trajectory of \eqref{DCP: BQ-form} towards $\calS_i$. By \textit{drive towards $\calS_i$} we mean: let $\calW \subset \partial \calC$ be a small neighborhood of $\calS_i$ such that $\nabla f_h(\bfx)^{\top} \bfG(\bfx)\bfw_p < 0, \bfF_u(\bfx) \parallel \bfG(\bfx)\bfw_p, f_h(\bfx) > 0, \bfF_u(\bfx) \neq \mathbf{0}$ for all $\bfx \in \calW$ and $\calW \cap \calQ \subseteqq \calW$. However, if we are driving the trajectory of \eqref{DCP: BQ-form} towards $\calS_i \setminus \bar{\calI}$, then we must have $\nabla f_h(\bfx) \bfF_u(\bfx) < 0$ for all $\bfx \in \calS_i \setminus \bar{\calI}$, indicating that there exists a small neighborhood $\calV$ of $\calS_i \setminus \bar{\calI}$ such that $\nabla f_h(\bfx) \bfF_u(\bfx) < 0, \forall \bfx \in \calV$, as a result, we have $\bfF_u(\bfx) \parallel^+ \bfG(\bfx)\bfw_p, \forall \bfx \in \calV \cap \calW$, showing that $\bfF_u(\bfx)$ and $\bfG(\bfx)\bfw_p$ are in the same direction, which contradicts the definition of $\calS_i$ since there exists an $\epsilon^*$ such that $\calB_{\epsilon^*}(\bfx) \cap \calV \subseteq \calV, \forall \bfx \in \calS_i \setminus \bar{\calI}$ and we will have $\calB_{\epsilon^*}(\bfx) \cap \calX_i = \emptyset, \forall \bfx \in \calS_i \setminus \bar{\calI}$. So, we will have non-removable $\calQ$ on the trajectory of \eqref{DCP: BQ-form} only if we wish to drive our system towards $\calS_i \cap \bar{\calI}$.

%%%%%%%%%%%%%%%%%%%%%%%%%%%%16/09/2022%%%%%%%%%%%%%%%%%%%%%%%%%%%%%

\section{Appendix}
Another version of Proposition~\ref{prop: DCP_uniqueness}.
\begin{proposition} \label{prop: DCP_Uniq_Lip}
    Consider the DCP in \eqref{criteria: index-zero_DCP}. Assume that the functions $\bfA, \bfq$ and $\bff$ are locally Lipschitz continuous. Moreover, 
	assume that the matrix $\bfA(\bfy)\in \R^{2\times 2}$ has the form
	\begin{equation}\label{eq: Amatrix_alt}
	\bfA(\bfy) = \left[ \begin{matrix}
			a(\bfy) & 0\\
			c(\bfy)\ & d(\bfy)
		\end{matrix} \right],
	\end{equation}
	with elements satisfying either:
	\begin{enumerate}
	    \item[i)] $a(\bfy_0)$ and $d(\bfy_0)>0$, or
	    \item[ii)] $a(\bfy_0) = 0, d(\bfy_0) > 0$ and $q_1(\bfy_0) > 0$. 
	\end{enumerate}
	If either i) or ii) holds, then the DCP \eqref{criteria: index-zero_DCP} is equivalent to an ODE with a locally Lipschitz right-hand side. 
\end{proposition}
\begin{proof}
    We prove the result under assumption i) first.  
    From \eqref{eq:Amatrix} and the continuity assumptions on the problem data, it follows that $\bfA(\bfy)$ is a $P$ matrix in a neighborhood $\mathcal{V}$ of $\bfy_0$. This implies that the solution $\bfz(\bfy)$ of $\mathrm{LCP}(\bfA(\bfy), \bfq(\bfy))$ is unique for all $\bfy \in \mathcal{V}$. 
    Define the index set 
    $$
      \alpha(\bfy) = \{i \in\{1,2\}| z_i(\bfy) > 0\} 
    $$
    and let $\alpha_0 = \alpha(\bfy_0)$. 
    
    If $\bfq(\bfy_0) > \mathbf{0}$, then using again the continuity assumption, it follows that $\bfq(\bfy)>\mathbf{0}$ in a neighborhood of $\bfy_0$. Without loss of generality, $\bfq(\bfy)>\mathbf{0}$ for all $\bfy\in \mathcal{V}$. It follows that for all $\bfy\in \mathcal{V}$, $\bfz(\bfy) = \mathbf{0}$ is the unique solution of $\mathrm{LCP}(\bfq(\bfy), \bfA(\bfy))$ and therefore the initial value DCP \eqref{criteria: index-zero_DCP}  is locally equivalent to the initial value ODE
    \begin{equation}\label{eq:auxODE_alt}
      \dot{\bfy} = \bff(\bfy, \mathbf{0}), \; \bfy(\mathbf{0}) = \bfy_0.
    \end{equation}
    
    If $\bfq(\bfy_0) > \mathbf{0}$ does not hold and $\alpha_0\ne \emptyset$. To prove the equivalence between the DCP and a locally Lipshitz ODE, we will use Theorem 7.3.7  and Theorem 7.3.9 from \cite{PangLCP}. This equivalence is guaranteed if $\bfz(\bfy_0)$ is a strongly stable solution of 
    $\mathrm{LCP}(\bfq(\bfy_0), \bfA(\bfy_0))$. To show this, we use condition c) of Theorem 7.3.7, \cite{PangLCP}, i.e., that the sub-matrix  $\bfA_{\alpha_0 \alpha_0}(\bfy_0)$ is non-singular and its Schur complement, $N_0$ is a $P$-matrix. This holds since 
    \begin{itemize}
        \item[-] for $\alpha_0=\{1,2\}$, 
        $\bfA_{\alpha_0\alpha_0}(\bfy_0)=\bfA(y_0)$ is non-singular,
        \item[-] for $\alpha_0=\{1\}$, $\bfA_{\alpha_0\alpha_0}(\bfy_0)= a(y_0)>0$ and
        $N_0 = d(y_0)>0$,
        \item[-] for $\alpha_0=\{2\}$, $\bfA_{\alpha_0\alpha_0}(\bfy_0)= d(y_0)>0$ and
        $N_0 = a(y_0)>0$.
    \end{itemize}

    If $\bfq(\bfy_0) = \mathbf{0}$, we need to prove $\bfz(\bfy_0)$ is locally Lipschitz for all $\bfy_0 \in \calH \coloneqq \{\bfy \mid a(\bfy_0), d(\bfy_0) > 0, \bfq(\bfy) = 0 \}$. First, $a(\bfy_0), d(\bfy_0) > 0$ implies $\bfA(\bfy_0)$ is non-singular for all $\bfy_0 \in \calH$. As a result, we could obtain $\bfz$ in closed-form expression $\bfz(\bfy_0) = \frac{1}{a(\bfy_0)d(\bfy_0)}[d(\bfy_0) q_1(\bfy_0), a(\bfy_0)q_2(\bfy_0) - c(\bfy_0)q_1(\bfy_0)]^{\top}$, so $\bfz(\bfy_0) = \mathbf{0}$, for all $\bfy_0 \in \calH$, which completes our proof of uniqueness.
    Since $a(\bfy_0)d(\bfy_0)$ is real valued and greater than zero for all $\bfy_0 \in \calH$, its reciprocal $\frac{1}{a(\bfy_0)d(\bfy_0)}$ is locally Lipschitz for all $\bfy_0 \in \calH$. As a result, $\bfz(\bfy_0)$ is locally Lipschitz for all $\bfy_0 \in \calH$. This completes the proof under assumption i).
    %\textit{Fact 1.} If $f_1$ and $f_2$ are locally Lipschitz continuous on a set $I$, then $f_1 + f_2$, $f_1f_2$, are each locally Lipschitz continuous on $I$. Furthermore, if $f_3$ is real valued, then in a neighborhood of any point $\bfx \in I$ where $f_3(\bfx) \neq 0$, $1/f_3$ is locally Lipschitz.
    
    To prove the result under assumption ii), we note that, due to the continuity assumptions, we have $q_1(\bfy) > 0$, for all $\bfy$ in a neighborhood $\mathcal{V}$ of $\bfy_0$. To satisfy the complementarity constraint, we need $z_1(\bfy)q_1(\bfy) = 0$. Since $q_1(\bfy) >0$ for all $\bfy \in \mathcal{V}$, $z_1(\bfy) = 0$ is the unique LCP solution and therefore $z_1(\bfy_0)$ is locally Lipschitz. The $\bfA$ matrix in \eqref{eq: Amatrix_alt} then reduces to a scalar $d(\bfy) > 0$ and we could consult our proof under assumption i) directly. \qedhere
\end{proof}

%The following is my proof about the local Lipschitzness for $\bfy \in \calH \coloneqq \{ \bfy \in \calD: \bfq(\bfy) = 0 \}$. $\calD$ is our domain of interest where $\bfA, \bfq$ and $\bff$ are locally Lipschitz continuous, $a(\bfy) = 0$ if and only if $q_1(\bfy) < 0$ and $a(\bfy) > 0$ otherwise, $d(\bfy) > 0$ for all $\bfy \in \calD$. Noted that we no longer assume $\| \bfq(\bfy) \| \neq 0$. Proposition~\ref{prop: DCP_Uniq_Lip} already address the case where we have $\| \bfq(\bfy) \| \neq 0$, now we need to prove $\bfz$ are still locally Lipschitz for all $\bfy \in \calH$.

%First, $\bfq(\bfy) = \mathbf{0}$ implies $a(\bfy), d(\bfy) > 0$, so $\bfA(\bfy)$ is non-singular for all $\bfy \in \calH$. As a result, we could obtain $\bfz$ in closed-form expression $\bfz(\bfy) = \bfA^{-1}(\bfy) \bfq(\bfy)$ with 
%$$
%\bfA^{-1} = \frac{1}{a(\bfy)d(\bfy)} \left[ \begin{matrix} d(\bfy) & 0 \\ -c(\bfy)\ & a(\bfy) \end{matrix} \right].
%$$
%Now $\bfz(\bfy) = \frac{1}{a(\bfy)d(\bfy)}[d(\bfy) q_1(\bfy), a(\bfy)q_2(\bfy) - c(\bfy)q_1(\bfy)]^{\top}$, so $\bfz(\bfy) = \mathbf{0}$, for all $\bfy \in \calH$, which completes our proof of uniqueness. 
%To the Lipschitz result, we need the following fact. \\
%\textit{Fact 1.} If $f_1$ and $f_2$ are locally Lipschitz continuous on a set $I$, then whenever their sum, $f_1 + f_2$, or product, $f_1f_2$, makes sense, they are each locally Lipschitz continuous on $I$. Furthermore, if $f_3$ is real valued, then in a neighborhood ofany point $\bfx \in I$ where $f_3(\bfx) \neq 0$, the reciprocal $1/f_3$ is locally Lipschitz.

%We have $\bfz(\bfy)$ locally Lipschitz for all $\bfy \in \calH$ accordig to \textit{Fact 1}, which completes our proof.

\begin{theorem} \label{trem: sol_DCP-BQ}
	Assume $\calL_{\bfG}V(\bfx) \neq \mathbf{0}$, $\forall \bfx \in \calE \coloneqq \{\bfx \in \calC \setminus \{\mathbf{0}\} \mid F_V(\bfx)=0 \}$
    %\NA{Give this set a name, e.g., $\calE$ so we do not have to repeat this long expression.} 
	%\BG{Probably it is more clear if we state the domain where we require non-zero values as $\forall \bfx \in \left(\calC\setminus \bf0\right)\cap\{\bfx \in \R^n : \bfF_V(\bfx) = 0 \}$}
    %\YY{Actually we could have $F_V(\bfx) = 0$ according to our Definition~\ref{CLF}, so I need to add this assumption to guarantee the uniqueness of our solution.}
    and $\bfw_l$ and $\bfw_h$ are chosen to satisfy $-\calL_{\bfG}V(\bfx) \cdot \bfw_l > 0$, $\forall \bfx \in \left(\calC\setminus \bf0\right)\cap\{\bfx \in \R^n : 
    \calL_{\bfG}V(\bfx) \neq \mathbf{0}\}$
    %\BG{The same type of remark as before: $\forall \bfx\in\left(\calC\setminus \bf0\right)\cap\{\bfx \in \R^n : 
    %\calL_{\bfG}V(\bfx) \neq \mathbf{0}\}$}
    and $\mathcal{L}_{\bfG}h(\bfx) \cdot \bfw_h > 0$.
    Then for all $\bfx \in \calC \setminus \{ \mathbf{0} \}$, the solution of \eqref{DCP: CLC}-\eqref{DCP: CBC} is unique and has a closed-form:
	%
	\begin{equation} 
		\label{sol: DCP-BQ}
		\begin{aligned}
			&\bar{u}_l =  -\frac{F_V(\bfx)}{\mathcal{L}_{\bfG}V(\bfx) \cdot \bfw_l}, \ F_V(\bfx) \geq 0, \\
            &\bar{u}_l =  0, \ F_V(\bfx) < 0, \\
			&\bar{u}_h = \left(-\frac{F_h(\bfx) + \mathcal{L}_{\bfG}h(\bfx) \cdot \bfw_l \bar{u}_l }{\mathcal{L}_{\bfG}h(\bfx) \cdot \bfw_h}\right)_+
		\end{aligned}
	\end{equation}
	%
	where $(\cdot)_+$ denotes $\max(\cdot,0)$. Moreover, if Assumption~\ref{assumption: lipschitz} holds, then $\bar{u}_l$ and $\bar{u}_h$ are locally Lipschitz continuous for all $\bfx \in \calC \setminus \{ \mathbf{0} \}$.
	\begin{proof} 
	    %\begin{comment}
	    %We notice that
		%$\left[ \begin{matrix}
		%	-\mathcal{L}_{\bfG}V(\bfx) \cdot \bfw_l & 0\\
		%	\mathcal{L}_{\bfG}h(\bfx) \cdot \bfw_l & \mathcal{L}_{\bfG}h(\bfx) \cdot %\bfw_h
		%\end{matrix} \right]$
		%is a $P$-matrix, thus the uniqueness result follows directly from Proposition~\ref{prop: DCP_uniqueness}. 
		%\end{comment}
        Rewrite \eqref{DCP: CLC}-\eqref{DCP: CBC} as follows $0 \leq \bfz(\bfx) \perp \bfA(\bfx) + \bfq(\bfx) \geq 0$ with $\bfq(\bfx) = [-F_V(\bfx), F_h(\bfx) + \mathcal{L}_{\bfG}h(\bfx) \cdot \bfw_l\bar{u}_l]^{\top}$ to reflect \eqref{criteria: index-zero_DCP}. For the case $\calL_{\bfG}V(\bfx) \neq \mathbf{0}$, we have 
        $\bfA(\bfx) = \left[ \begin{matrix}
			-\mathcal{L}_{\bfG}V(\bfx) \cdot \bfw_l & 0\\
			\mathcal{L}_{\bfG}h(\bfx) \cdot \bfw_l & \mathcal{L}_{\bfG}h(\bfx) \cdot \bfw_h
		\end{matrix} \right]$
		with $a(\bfx) = -\mathcal{L}_{\bfG}V(\bfx) \cdot \bfw_l > 0$ and $d(\bfx) = \mathcal{L}_{\bfG}h(\bfx) \cdot \bfw_h > 0$.
        %\NA{This is too brief. What is $\bfA(\bfx)$? You also need to appeal to Proposition~\ref{prop: DCP_uniqueness}.}
        For the case $\calL_{\bfG}V(\bfx) = \mathbf{0}$, we must have $-F_V(\bfx) > 0$ according to our assumption on $\calL_{\bfG}V(\bfx)$ and Definition~\ref{CLF}. Thus, to satisfy the complementarity constraint, we must have $\bar{u}_l =  0$. To solve $\bar{u}_h$ in this case, we simply have 
        $\bfA(\bfx) = d(\bfx) = \mathcal{L}_{\bfG}h(\bfx) \cdot \bfw_h > 0$.
        %reduce our matrix $\bfA$\NA{This should be bold and it is not necessary to repeat} to $\bfA(\bfx) = d(\bfx) = \mathcal{L}_{\bfG}h(\bfx) \cdot \bfw_h > 0$.
        %\NA{This sentence is too long. Break it up into two. Good writing uses one sentence for one piece of information.}.
        %It follows from  Theorem 7.3.7 in \cite{PangLCP}, that  for any $\bfx \in \calC \setminus \{ \mathbf{0} \}$ the unique solution of the corresponding LCP is strongly regular. 
        As a result, the uniqueness result for the DCP \eqref{DCP: BQ-form} follows now directly from Proposition~\ref{prop: DCP_uniqueness}.

        If $\bar{u}_l$ is locally Lipschitz for all $\bfx \in \calC \setminus \{ \mathbf{0} \}$, then the local Lipschitzness of $\bar{u}_h$ follows directly from \cite[Theroem 8]{xu2015robustness}, this theorem also applies to the case where we have $\calL_{\bfG} V(\bfx) \neq \mathbf{0}$. However, there exists $\calH \subseteq \calC \setminus \{ \mathbf{0} \}$ such that $\calL_{\bfG} V(\bfx) = \mathbf{0}$, $\forall \bfx \in \calH$. As we mentioned above, $\calL_{\bfG} V(\bfx) = \mathbf{0}$ implies $F_V(\bfx) < 0$ and $\bar{u}_l = 0$, as a result, if we have $\bar{u}_l = 0$ in a neighborhood around each $\bfx \in \calH$, then we will have $\bar{u}_l$ locally Lipschitz for all $\bfx \in \calH$. Consider $\bar{\bfx} \in \calH$, let $\calU$ denote the set such that $\exists L \in \bbR_{> 0}: | F_V(\bar{\bfx}) - F_V(\bfx) | \leq L \| \bar{\bfx} - \bfx \|_2, \forall \bfx \in \calU$ and define $\delta = \min_{\bfx \in \calU} \| \bar{\bfx} - \bfx \|$, $\Delta \in \bbR_{> 0}: \Delta < \textrm{min}(\delta, | F_V(\bar{\bfx})| / L)$. Then for all $\bfx \in \calB_{\Delta}(\bar{\bfx})$, where $\calB_{\Delta}(\bar{\bfx})$ denotes an abstract ball centered at $\bar{\bfx}$ with radius $\Delta$, formally defined by  $\calB_{\Delta}(\bar{\bfx}) \coloneqq \{ \bfx \in \bbR^n: \| \bar{\bfx} - \bfx \|_2 \leq \Delta \}$, we have $| F_V(\bar{\bfx}) - F_V(\bfx) | \leq L \Delta < | F_V(\bar{\bfx})|$. Recall $F_V(\bar{\bfx}) < 0$, thus $F_V(\bar{\bfx}) < F_V(\bar{\bfx}) - F_V(\bfx) < -F_V(\bar{\bfx})$, which yields: $2F_V(\bar{\bfx}) < F_V(\bfx) < 0$, $\forall \bfx \in \calB_{\Delta}(\bar{\bfx})$. It follows that $\bar{u}_l = 0$, $\forall \bfx \in \calB_{\Delta}(\bar{\bfx})$ and as a result, $\bar{u}_l$ locally Lipschitz for all $\bfx \in \calH$.
        
		Also, once we obtain the closed-form expression of $\bar{u}_l$ from \eqref{DCP: CLC}, we could simplify \eqref{DCP: CBC} by substituting $\bar{u}_l$ with its closed-from expression and \eqref{DCP: CBC} will have the same structure as \eqref{DCP: CLC}. Thus we only consider \eqref{DCP: CLC} since \eqref{DCP: CBC} can be solved by the same procedure: If $\bar{u}_l = 0$ holds, then $-F_V(\bfx) \geq 0$ must hold. If $\bar{u}_l > 0$ holds, then $-F_V(\bfx) - \mathcal{L}_{\bfG}V(\bfx) \cdot \bfw_l\bar{u}_l = 0$ must hold, and we solve the equation above to obtain $\bar{u}_l = -\frac{F_V(\bfx)}{\mathcal{L}_{\bfG}V(\bfx) \cdot \bfw_l}$. However since we require $\bar{u}_l > 0$, $-F_V(\bfx) < 0$ must hold, thereby the solution of $\bar{u}_l $ is obtained for all state. %Therefore, the unique solution is explicitly formulated as $\bar{u}_l = ( -\frac{F_V(\bfx)}{\mathcal{L}_{\bfG}V(\bfx) \cdot \bfw_l} )_+$. 
	\end{proof}
\end{theorem}
